# Supplementary material for: ESVIO: Event-based Stereo Visual Inertial Odometry
Source: arXiv:2212.13184 source file (2024-03-11)
Supplement: Supplementary file 1 [file supplementary_materials.pdf]

# Supplementary Materials —— ESVIO: Event-based Stereo Visual Inertial Odometry


**Abstract**

The structure of this document is organized as follows: Section I introduces our self-collected dataset on the HKU campus. Section II supplementarily demonstrates the quantitative performance of our ESIO and ESVIO in the evaluation of rosbag and onboard quadrotor flight. Section III supplementarily demonstrates the qualitative performance of our ESIO and ESVIO in the DSEC dataset; the failure cases of ORB-SLAM3, VINS-Fusion, Ultimate SLAM in our self-collect dataset; The limitations of our ESVIO in the low-texture environment. Finally, in section IV, we conduct the performance comparison of our ESVIO with ORB-SLAM3 and Ultimate SLAM in offline quadrotor flight.


## I. Introduction of Self-collected Dataset

The self-collected dataset (Table I in [1]) contains stereo event data at 60HZ and stereo image frames at 30Hz with resolution in $346 \times 260$, as well as IMU data at 1000Hz. The timestamps between all sensors are synchronized in hardware. We also provide ground truth poses from a motion capture system VICON at 50Hz during the beginning and end of each sequence, which can be used for trajectory evaluation. To alleviate disturbance from the motion capture system's infrared light on the event camera, we add an infrared filter on the lens surface of the DAVIS346 camera. Note that this might cause the degradation of perception for both the event and image camera during the evaluation, but it can also further increase the challenge of our dataset for the only image-based method.

It is worth mentioning that this is a very challenging dataset for event-based VO/VIO, featuring aggressive motion and HDR scenarios. EVO [2], ESVO [3], Ultimate SLAM [4] are failed in most of the sequences. We think that parameter tuning is infeasible, therefore, we suggest the users use the same set of parameters during the evaluation. We hope that our dataset can help to push the boundary of future research on event-based VO/VIO algorithms, especially the ones that are really useful and can be applied in practice. For the convenience of the community, we also release the results of our methods, including the estimated 6-DoF pose and the ground truth, in the form of rosbag[1]. We figure out this solution for benchmark testing and performance comparison rather than re-run our source code.

## II. Quantitative Evaluation of our ESIO and ESVIO

### A. *Quantitative Evaluation on rosbag*

Different from the evaluated metric of the original paper, in this section, we also give the accuracy evaluation in absolute trajectory error (ATE) format. The accuracy is measured with ATE aligning the estimated trajectory with ground truth using 6-DOF transformation (in SE3), which is calculated by the tool [5]. TableI and TableII is the evaluation of our methods in self-collected dataset, Vector [6], and MVSEC [7], respectively. They are also corresponding to Table I and Table II in our original manuscript [1] respectively.

We also evaluate EVO [2] and ESVO [3] in our self-collected datasets, but they failed in all sequences. Therefore, we do not list them in TableI. This might be caused by three factors: Firstly, both EVO and ESVO have strict initialization requirements. For example, EVO requires running in a uniform scene for a few seconds to boost the system. Secondly, they are sensitive to parameter tuning, even in their open-source project, they use different parameters for different sequences in the same scenarios. We might fail to correctly tune parameters for their successful running. Finally, our dataset is so challenging that only reliable methods can perform well. As for the data sequence of MVSEC [7] and Vector [6], we list the result of EVO [2] and ESVO [3] in TableII, but they still fail in most of the sequences.

Please note that we think that parameter tuning is infeasible. Therefore, we evaluate our methods using fixed parameters for all sequences during the evaluations. We also use this criterion when evaluating other methods as a comparison. However, the generalization capability of [2] [3] is slightly poor, they need finely parameter tuning for different *rosbag*. We have tried our best to tune the parameter of these methods during the evaluation, however, their performance is still unsatisfactory. Meanwhile, the performance of ESVO [3] in Table II is worse than that of the original paper, which should be caused by the intercept of the time period from the original *rosbag*. For example, ESVO [3] only can work well during [0-27s] of sequence *Indoor Flying 3* (the total duration is 94s), but it has significant drifts after 27s. Instead, we use the whole sequence *Indoor Flying 3* without any timestamp modification. The absolute mean error of the original paper and our results are 0.19m and 0.91m respectively.

Supplementary update: We found that [8] also evaluated their method in *school-dolly* and *school-scooter* sequences. However, their video only shows the performance of their proposed method during [0-10s] of sequence *school-dolly* (the total duration is 108s) and [0-8s] of sequence *school-scooter* (the total duration is 45s). Therefore, their evaluations in these two data sequences

[1]https://github.com/arclab-hku/Event_based_VO-VIO-SLAM/blob/main/Results_for_comparison.md

are not complete. Meanwhile, their algorithm cannot run in real-time and need to slow down the playback of the rosbag. While our ESVIO can estimate poses accurately in real-time even in high-resolution cameras.

Besides, we emphasize real-time performance when evaluating our methods, while the computational burden of EVO [2] and ESVO [3] is so large that we had to slow down the *rosbag* such as $\times 0.2$ or $\times 0.5$ data-speed, during the evaluations. Other compared methods are evaluated using the original data speed of the *rosbag*. The running time of our methods can be seen in the original manuscript. We also provide a visual comparison between our method and the other methods in the accompanying video, and all the video records of our ESVIO during the evaluations can be also obtained on our website.

We also evaluate our ESIO and ESVIO in DSEC [9] dataset, however, since the DSEC dataset does not provide the ground truth 6-DoF poses, we cannot obtain the quantitative results. Therefore, we only show the qualitative results which would be further discussed in section III-A.

TABLE I. Accuracy Comparison of Our ESVIO on HKU Dataset

| Sequence | ORB-SLAM3 [10] Stereo VIO | VINS-Fusion [11] Stereo VIO | USLAM [12] Mono EIO | USLAM [4] Mono EVIO | PL-EVIO [13] Mono EVIO | **Our ESIO Stereo EIO** | **Our ESIO+ Stereo EIO** | **Our ESVIO Stereo EVIO** |
|---|---|---|---|---|---|---|---|---|
| hku_agg_translation | 0.095 | 0.069 | 10.41 | 0.38 | **0.048** | 0.38 | 0.35 | 0.063 |
| hku_agg_rotation | 0.23 | 0.88 | *failed* | 2.06 | 0.15 | 0.87 | 0.51 | **0.11** |
| hku_agg_flip | **0.14** | 0.45 | 4.32 | 2.66 | 0.15 | 1.47 | 1.23 | **0.14** |
| hku_agg_walk | *failed* | *failed* | *failed* | 1.75 | 0.37 | 1.31 | 1.14 | **0.27** |
| hku_hdr_circle | 0.083 | 2.52 | 0.46 | 0.66 | **0.068** | 0.69 | 0.23 | 0.081 |
| hku_hdr_slow | 0.086 | 0.073 | *failed* | 1.52 | 0.069 | 0.16 | 0.17 | **0.059** |
| hku_hdr_tran_rota | 0.20 | 0.075 | *failed* | 1.74 | 0.068 | 0.55 | 0.60 | **0.065** |
| hku_hdr_agg | 0.28 | 1.18 | *failed* | 2.40 | 0.14 | 2.27 | 1.37 | **0.10** |
| hku_dark_normal | *failed* | 0.80 | *failed* | 2.01 | 1.25 | **0.28** | 0.32 | 0.39 |
| Average | 0.16 | 0.76 | 5.06 | 1.69 | 0.26 | 0.89 | 0.66 | **0.14** |

**EIO means purely event-based VIO, EVIO means event-based VIO with image-aided*

TABLE II. Accuracy Comparison of Our ESVIO with Other Image-based or Event-based Methods

| Sequence | | ORB-SLAM3 [10] Stereo VIO | VINS-Fusion [11] Stereo VIO | EVO [2] Mono EO | ESVO [3] Stereo EO | Ultimate SLAM [4] Mono EVIO | PL-EVIO [13] Mono EVIO | **Our ESVIO Stereo EVIO** |
|---|---|---|---|---|---|---|---|---|
| VECtor [6] | corner-slow | 0.012 | 0.013 | 0.035 | 0.039 | 0.039 | 0.017 | **0.012** |
| | robot-normal | 0.029 | **0.023** | 0.13 | *failed* | 0.047 | 0.027 | 0.043 |
| | robot-fast | 0.15 | *failed* | *failed* | *failed* | 0.35 | **0.037** | 0.042 |
| | desk-normal | **0.039** | 0.040 | *failed* | *failed* | 0.19 | 0.31 | 0.052 |
| | desk-fast | 0.099 | 0.10 | *failed* | *failed* | 0.34 | 0.043 | **0.042** |
| | sofa-normal | **0.044** | 0.038 | *failed* | 0.53 | 1.72 | 0.058 | 0.047 |
| | sofa-fast | 0.064 | 0.17 | *failed* | *failed* | 0.76 | **0.050** | 0.052 |
| | mountain-normal | **0.026** | 0.30 | *failed* | *failed* | 0.27 | 0.32 | 0.044 |
| | mountain-fast | 0.52 | *failed* | *failed* | *failed* | 1.02 | **0.031** | 0.039 |
| | hdr-normal | 0.019 | 0.038 | *failed* | *failed* | 0.17 | 0.12 | **0.017** |
| | hdr-fast | 0.040 | 0.055 | *failed* | *failed* | 0.48 | **0.036** | 0.039 |
| | corridors-dolly | **0.80** | 1.46 | *failed* | *failed* | *failed* | 1.23 | 0.88 |
| | corridors-walk | 1.03 | 0.39 | *failed* | *failed* | *failed* | 0.72 | **0.34** |
| | school-dolly | 0.92 | 1.79 | *failed* | 13.71 | *failed* | 3.11 | **0.53** |
| | school-scooter | 0.75 | **0.56** | *failed* | 9.83 | 6.83 | 1.39 | 0.63 |
| | units-dolly | 18.06 | 10.39 | *failed* | *failed* | *failed* | 13.82 | **8.12** |
| | units-scooter | 14.50 | 11.47 | *failed* | *failed* | *failed* | 11.66 | **6.64** |
| MVSEC [7] | Indoor Flying 1 | 1.42 | 0.40 | 1.36 | 1.07 | *failed* | 0.36 | **0.25** |
| | Indoor Flying 2 | 1.70 | 2.10 | *failed* | 1.10 | *failed* | 0.30 | **0.30** |
| | Indoor Flying 3 | 1.54 | 0.39 | 1.37 | 0.91 | *failed* | 0.34 | **0.25** |
| | Indoor Flying 4 | 0.58 | 0.30 | *failed* | *failed* | **0.23** | 0.44 | 0.46 |

## *B. Quantitative Evaluation on Onboard Quadrotor Flighting*

Apart from the evaluation on rosbag, we also test our proposed method in the quadrotor platform. More details about this evaluation can be seen in our original manuscript [1]). We show the relative pose error (RPE) of the quadrotor flight using our ESVIO in the original manuscript. Here, we demonstrate the absolute pose error (APE) of our ESVIO compared with the ground truth in Fig.1.

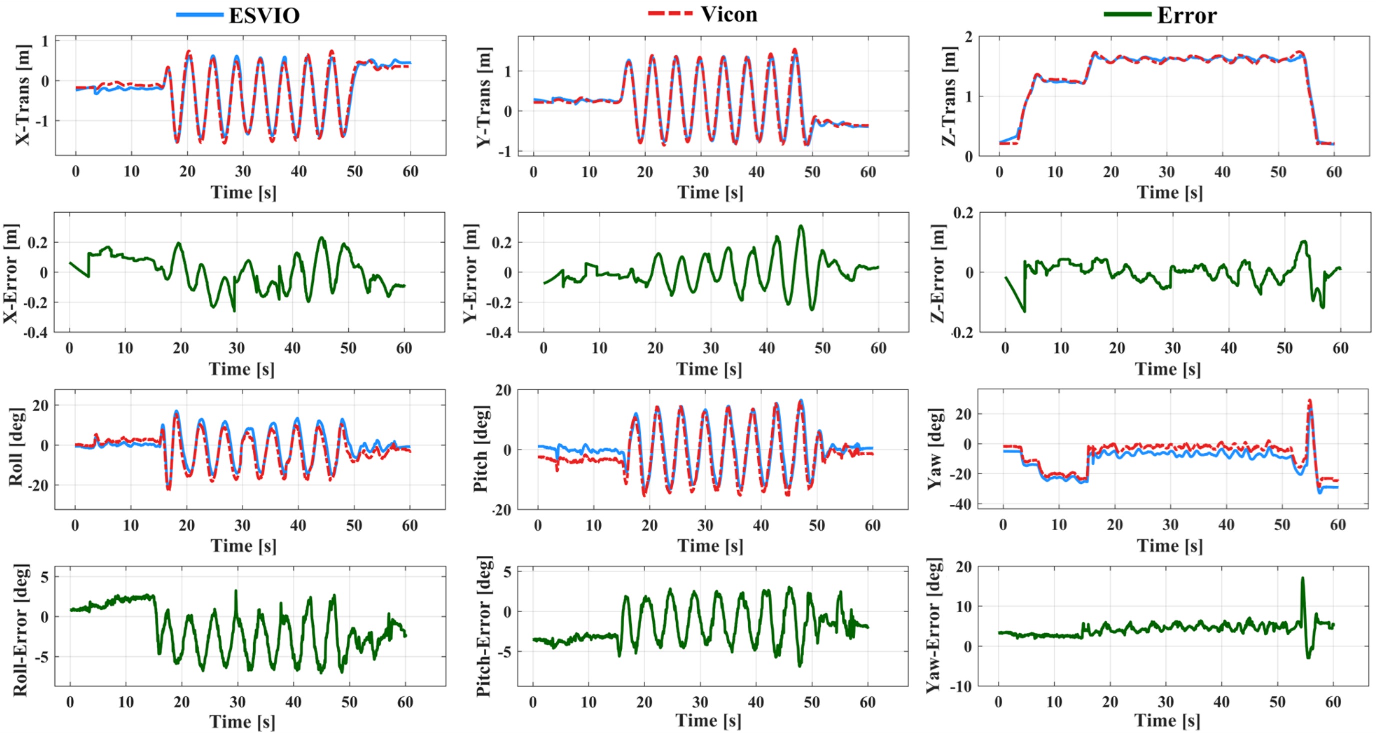


(a)

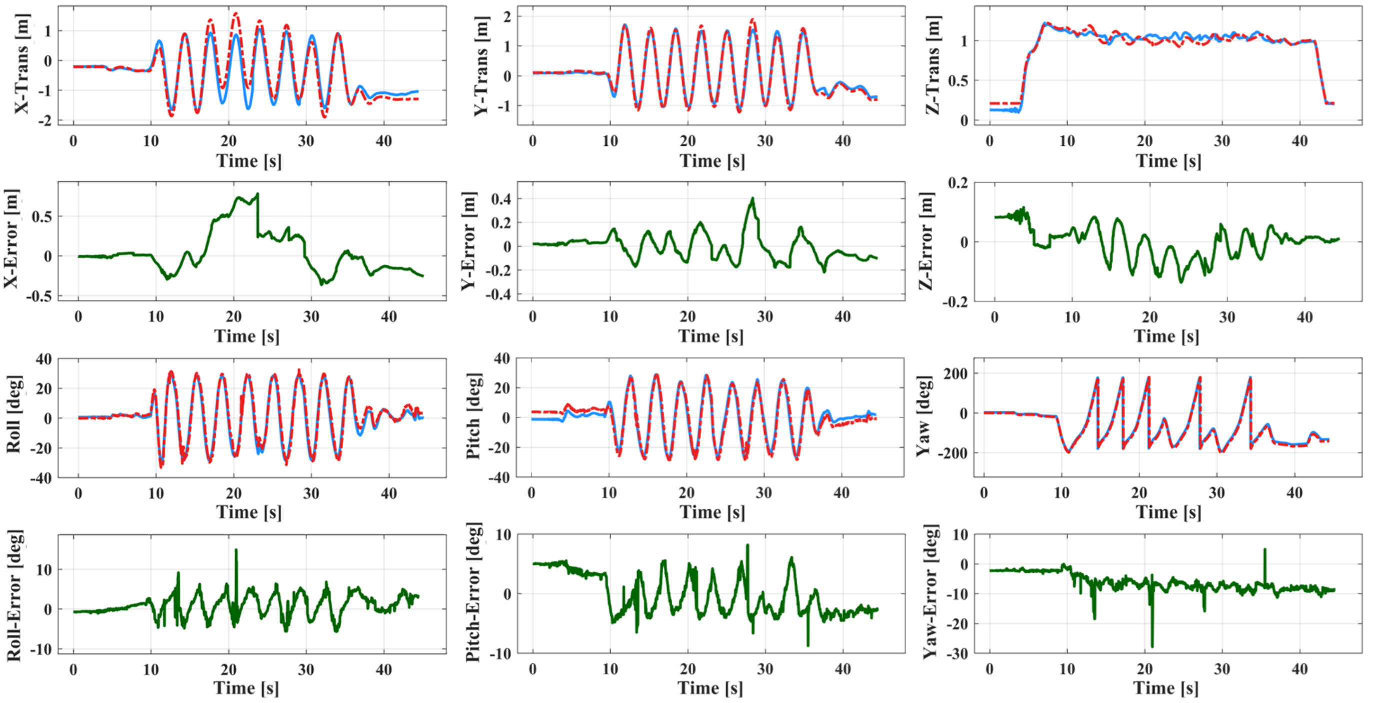


(b)

Fig. 1. The position (X, Y, Z), orientation (Roll, Pitch, Yaw), and the corresponding errors of our ESVIO compared with the VICON: (a) Onboard quadrotor flight in low-illumination conditions; (b) Onboard quadrotor flight in aggressive motion.

*1)* **Quadrotor Flight in HDR Scenarios:** We give the translational and rotational results of our ESVIO against the VICON in Fig. 1(a). The total trajectory length is 56.0m. The translation errors in the X and Y axis are within 0.3m, while the error in the Z axis is within 0.1m. For the rotational part, the error of roll and pitch are both within 6°. The error in yaw at 55s is larger than 10°, which is caused by rapid change in yaw at that moment resulting in the estimated pose being slightly slower than VICON. The root-mean-square error (RMSE) in HDR flight is 0.17m.

*2) Quadrotor Flight in Aggressive Motion:* In this section, the yaw angle of the commanded pattern is changed drastically, for aggressive motion. The performance of our ESVIO is quantitatively evaluated in Fig. 1(b). Note that it would have some outliers during the comparison with the VICON. For example, there is an error that is more than $10^\circ$ in the roll and yaw axis at 22s. This is caused by VICON's ball is not well observed during aggressive flight, resulting in an inaccurate measurement of the VICON at that moment. However, our reliable ESVIO state estimator still provides robust and accurate onboard pose feedback for the quadrotor. The RMSE of our ESVIO in this aggressive flight is 0.26m.

## III. Qualitative Evaluation of our ESIO and ESVIO

### *A. Qualitative Evaluation on DSEC Dataset*

To show the performance of our proposed methods in large-scale scenes, apart from outdoor large-scale HKU campus evaluation, we also perform the qualitative evaluation on the public driving dataset DSEC [9]. Since the DSEC dataset does not provide the ground-truth of the trajectory, we cannot evaluate our proposed methods quantitatively. The data sequence of DSEC was collected from stereo event cameras mounted on a driving car with 640 × 480 resolution. Driving scenarios are challenging for event-based sensors because forward motions typically produce considerably fewer events in the center of the image (where apparent motion is small) than in the periphery. Additionally, the higher sensor resolution (640 × 480), the large-scale outdoor scenes, and the dynamic objects (moving cars) are also challenging. Thanks to the robustness of our proposed method, both our ESIO (only event+IMU) and ESVIO (event+image+IMU) can perform fairly good results (shown in Fig. 2).

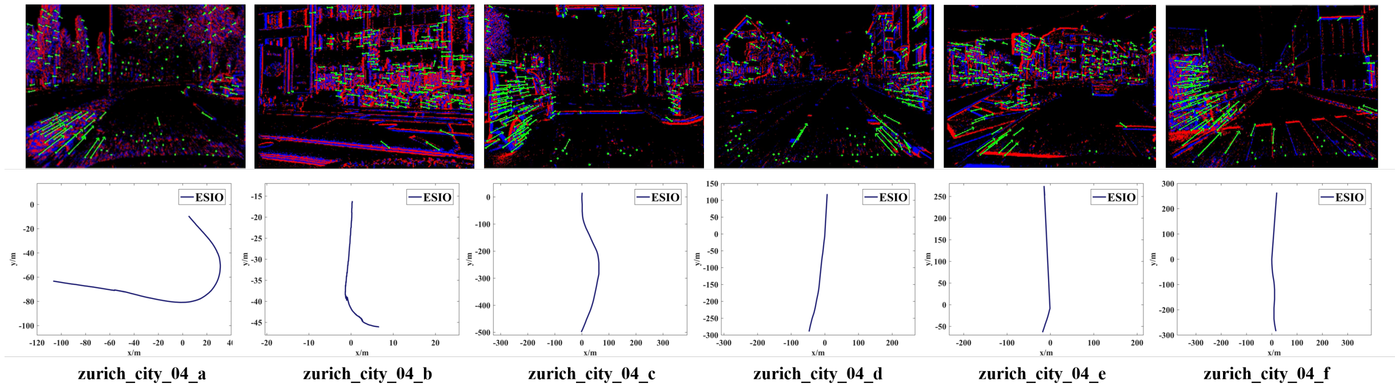


(a) ESIO

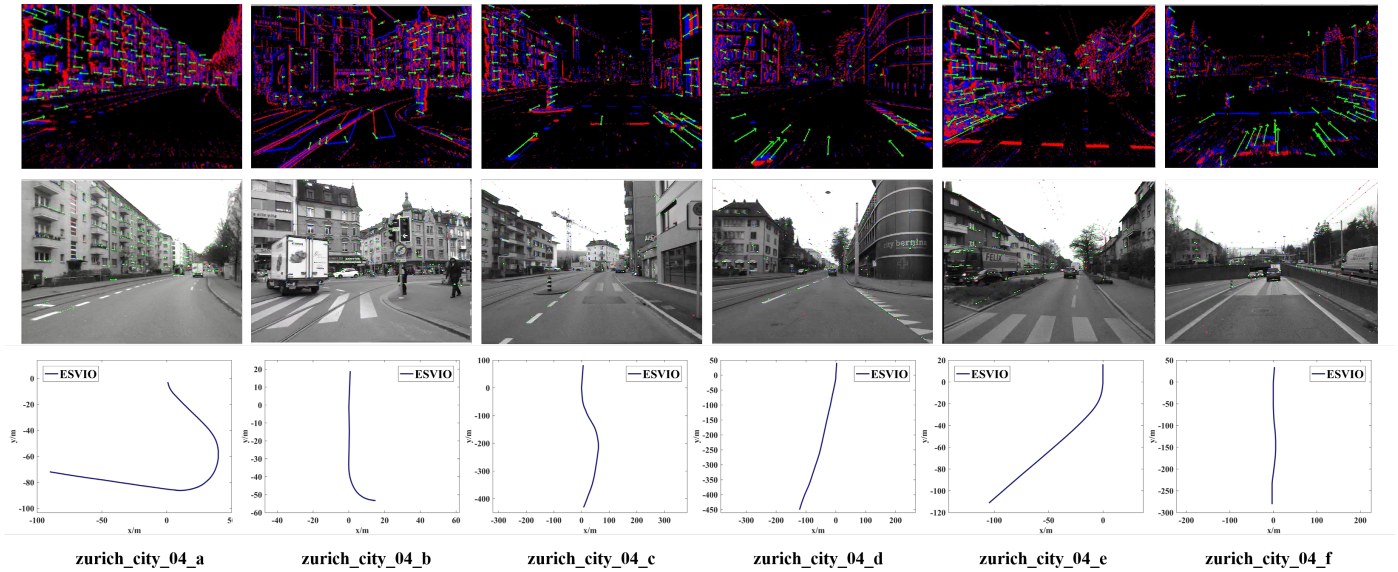


(b) ESVIO

Fig. 2. Since the DSEC dataset does not provide the ground truth 6-DoF poses, we only show the qualitative results, the tracking performance of event-based and image-based features, of (a) ESIO and (b) ESVIO for the DSEC dataset sequences zurich_city_04_a to zurich_city_04_f.

Note that Ref. [3] and [14] also evaluate their method in DSEC, however, they can not run in real-time and need to slow down the playback of the rosbag. While both our ESIO and ESVIO can perform in real-time and have good results even in very heavy events load. All the evaluations of our proposed method are recorded in videos[2].

What's more, the data sequence of different sensors in DSEC is divided and in different data formats, which is difficult to use for VO/VIO/SLAM researchers. Therefore, we convert them into the same rosbag which might be easier for event-based VIO evaluation. The processing code and the data can be also available on our project website.

### *B. Qualitative Evaluation on HKU / self-collected Dataset*

In this section, we visual the failure cases of ORB-SLAM3 [10], VINS-Fusion [11], and Ultimate-SLAM [4] in our self-collected data sequence. As can be seen in Table I, both our ESIO and ESVIO have good performance, especially for the sequence hku_agg_walk and hku_dark_normal, our ESVIO and ESIO still can produce reliable and accurate pose estimation even when the state-of-the-art image-based VIO method fails. As can be shown in Fig.3(a), both the ORB-SLAM3 and VINS-Fusion can not achieve reliable feature tracking under the aggressive motion due to motion blur, which causes the failure of the trajectory estimator. While our ESVIO performs satisfactory results compared with the ground truth from VICON. As for the evaluation in Fig.3(b), the ORB-SLAM3 can not extract any feature in the dark environment. As for the Ultimate SLAM, although it can detect some features in the event frame, it still cannot perform successfully feature tracking and data association in this situation. Therefore, both the ORB-SLAM3 and Ultimate SLAM fail in this case. While our proposed ESVIO can perform reliable feature detection and tracking in this harsh environment with good alignment with the ground truth.

It is worth mentioning that all the evaluations of our ESIO and ESVIO are recorded in video, which is available on our website, we refer the readers to the qualitative evaluation through consecutive videos rather than just through a single timestamp.

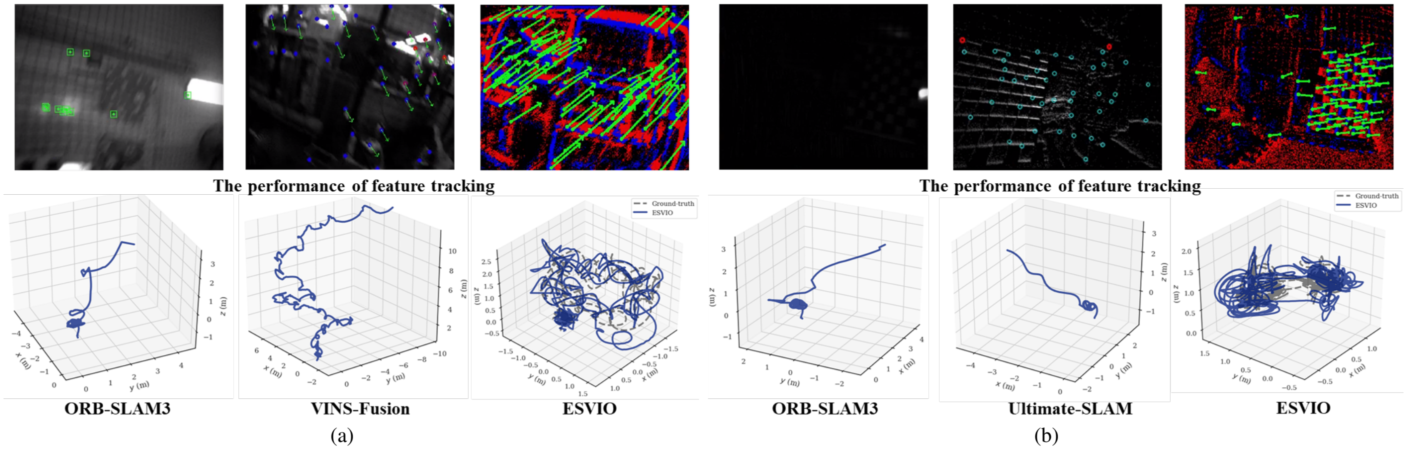


Fig. 3. The comparison of our ESVIO with ORB-SLAM3 [10], VINS-Fusion [11], and Ultimate SLAM [4] in our self-collected dataset. (a) The cases in hku_agg_walk sequences. (b) The cases in hku_dark_normal sequences.

### *C. Qualitative Evaluation on VECtor large-scale sequence*

As can be seen in TableII, although our ESVIO achieves fairly good results compared with the state-of-the-art image-based and event-based VIO, it still has limitations in the low-texture environment. For example, the scenarios in sequence *units-dolly* and *units-scooter* are so special that the visual-only method might be easy to degenerate or mismatch during the loop-closure detection. Most of the scenes in these two sequences are low-texture, which leads to few event generations, this might cause some trouble for the methods that depend on event streams. Thanks to our well-design event-corner feature management, and the framework of the tightly-couple event, image, and IMU data fusion, our proposed ESVIO still can achieve good results compared with the ground truth in most of the sequences. However, this still indicates that either event camera or standard camera has limitations, although event cameras play a complementary role to the traditional image-based method, multi-sensor fusion, especially vision-based and non-vision-based, should be developed to exploit the complementary advantage of different sensors.

What's more, as can be seen from the video record of the evaluation using our ESVIO (take the *school-scooter* [3] in Vector and *indoor_flying_1* [4] in MVSEC [7] as examples). The estimated trajectory of our ESVIO is very smooth rather than serrate-like

[2]https://b23.tv/6ByR30F
[3]https://b23.tv/pk7jdKp
[4]https://b23.tv/SmuzhgB

trajectory with shaking like Ref. [3] [14] [8]. Reliable and smooth state estimation is really important in onboard perception and localization. This is also the reason that we emphasize the real-time and robust capability of our proposed methods which can not only achieve satisfactory real-time performance but also ensures the practicality and reliable onboard quadrotor flight.

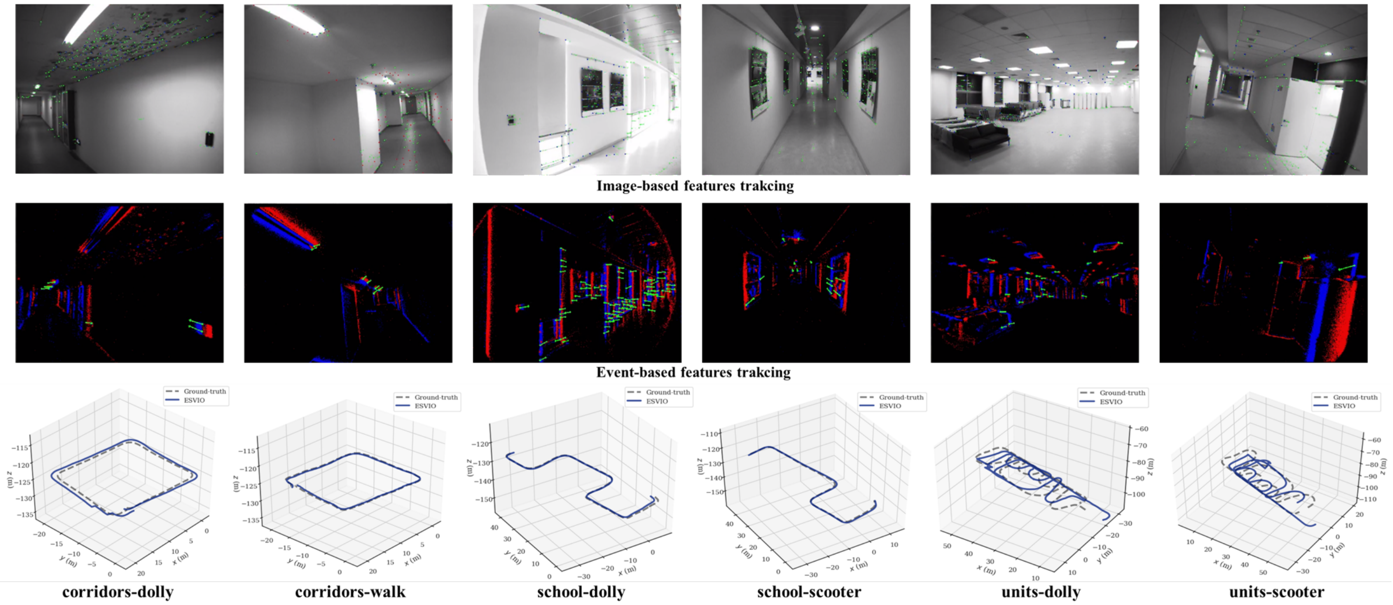


Fig. 4. Qualitative evaluation of our ESVIO in VECtor large-scale sequences. **Top:** The stereo image-based feature tracking performance; **Middle:** The stereo event-corner feature tracking performance; **Bottom:** The estimated trajectories produced by our ESVIO.

## IV. Performance Comparison on HDR offline Quadrotor Flight

In [1], we only demonstrate that using our ESVIO for onboard quadrotor flight. In this section, we conduct a new experiment that records the sensor data during quadrotor flight and then use it to compare the performance of our ESVIO, ORB-SLAM3 [10], and Ultimate SLAM [4]. Similar to [1], the state estimation from our ESVIO is used to provide onboard pose feedback control for the quadrotor. The quadrotor is commanded to follow a circular pattern eight times continuously during the experiment. The robust and accurate onboard state estimates of our ESVIO enable real-time feedback control. We record the rosbag which includes the ground truth from VICON, stereo event stream, stereo image, and IMU, for evaluation. As can be seen from the top two rows of Fig.5, in the condition of turning off the light, all the image-based features tracking is unreliable and rare in these three methods. However, thanks to our robust and reliable stereo event-corner feature detection and association, only our ESVIO can perform reliable and accurate state estimation. While both ORB-SLAM3 and Ultimate SLAM failed in the HDR quadrotor flight. The comparison of our ESVIO with other SOTA algorithms can be seen in the video[5].

## References

[1] P. Chen, W. Guan, and P. Lu, "Esvio: Event-based stereo visual inertial odometry," *arXiv preprint arXiv:2212.13184*, 2022.
[2] H. Rebecq, T. Horstschäfer, G. Gallego, and D. Scaramuzza, "Evo: A geometric approach to event-based 6-dof parallel tracking and mapping in real time," *IEEE Robotics and Automation Letters*, vol. 2, no. 2, pp. 593–600, 2017.
[3] Y. Zhou, G. Gallego, and S. Shen, "Event-based stereo visual odometry," *IEEE Transactions on Robotics*, 2021.
[4] A. R. Vidal, H. Rebecq, T. Horstschaefer, and D. Scaramuzza, "Ultimate slam? combining events, images, and imu for robust visual slam in hdr and high-speed scenarios," *IEEE Robotics and Automation Letters*, vol. 3, no. 2, pp. 994–1001, 2018.
[5] M. Grupp, "evo: Python package for the evaluation of odometry and slam," *Note: https://github. com/MichaelGrupp/evo Cited by: Table*, vol. 7, 2017.
[6] L. Gao, Y. Liang, J. Yang, S. Wu, C. Wang, J. Chen, and L. Kneip, "Vector: A versatile event-centric benchmark for multi-sensor slam," *IEEE Robotics and Automation Letters*, 2022.
[7] A. Z. Zhu, D. Thakur, T. Özaslan, B. Pfrommer, V. Kumar, and K. Daniilidis, "The multivehicle stereo event camera dataset: An event camera dataset for 3d perception," *IEEE Robotics and Automation Letters*, vol. 3, no. 3, pp. 2032–2039, 2018.
[8] K. Wang and K. Zhao, "Stereo event-based visual-inertial odometry," *arXiv preprint arXiv:2303.05086*, 2023.
[9] M. Gehrig, W. Aarents, D. Gehrig, and D. Scaramuzza, "Dsec: A stereo event camera dataset for driving scenarios," *IEEE Robotics and Automation Letters*, vol. 6, no. 3, pp. 4947–4954, 2021.
[10] C. Campos, R. Elvira, J. J. G. Rodríguez, J. M. Montiel, and J. D. Tardós, "Orb-slam3: An accurate open-source library for visual, visual–inertial, and multimap slam," *IEEE Transactions on Robotics*, 2021.

[5]https://b23.tv/ExrSI3M

[11] T. Qin, J. Pan, S. Cao, and S. Shen, “A general optimization-based framework for local odometry estimation with multiple sensors,” *arXiv preprint arXiv:1901.03638*, 2019.

[12] H. Rebecq, T. Horstschaefer, and D. Scaramuzza, “Real-time visual-inertial odometry for event cameras using keyframe-based nonlinear optimization,” in *British Machine Vision Conference (BMVC)*, 2017.

[13] W. Guan, P. Chen, Y. Xie, and P. Lu, “Pl-evio: Robust monocular event-based visual inertial odometry with point and line features,” *arXiv preprint arXiv:2209.12160*, 2022.

[14] Z. Liu, D. Shi, R. Li, and S. Yang, “Esvio: Event-based stereo visual-inertial odometry,” *Sensors*, vol. 23, no. 4, p. 1998, 2023.

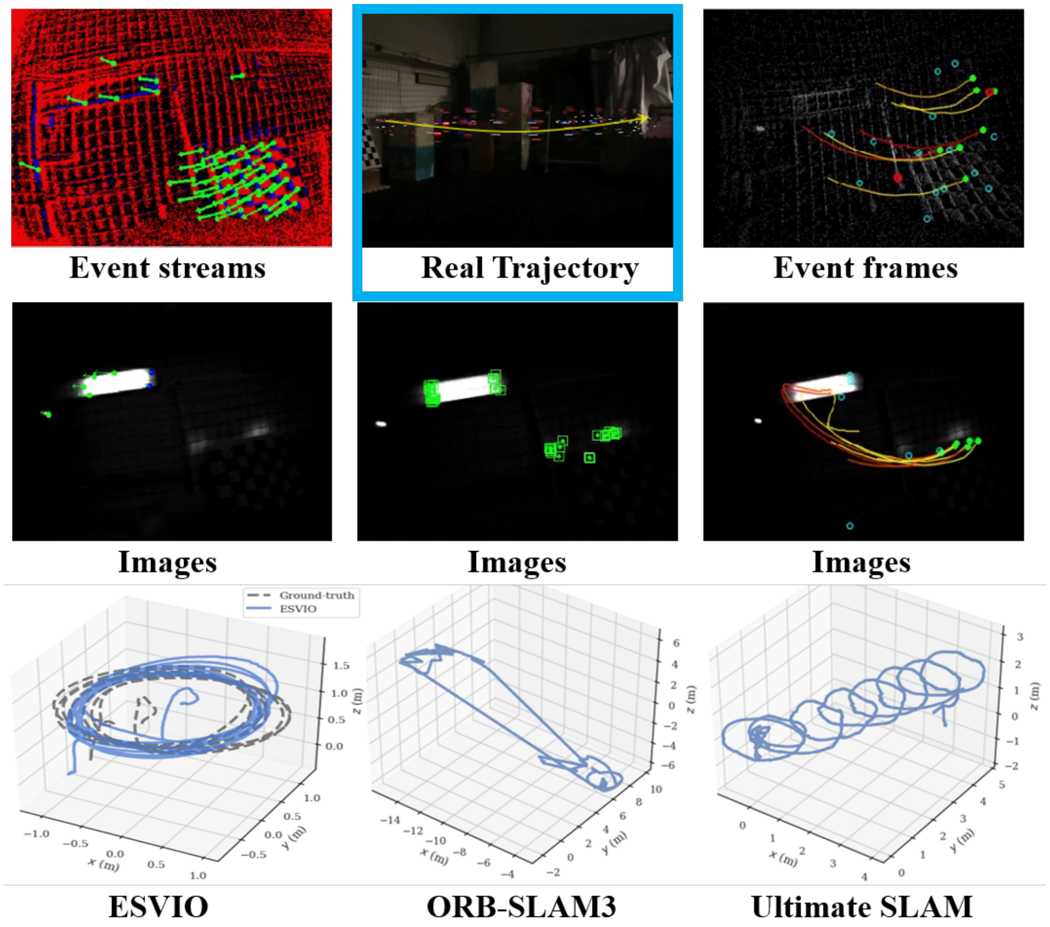


Fig. 5. Performance comparison of our ESVIO with ORB-SLAM3 and Ultimate SLAM in HDR offline quadrotor flight
